# Supplementary material for: Is Explanation the Cure? Misinformation Mitigation in the Short Term and Long Term
Source: arXiv:2310.17711 source file (2023-10-26)
Supplement: Supplementary file 1 [file Appendix.tex]

\section{Crowdsourcing Details}
\label{appendix:a}
\subsection{Procedure}
We sampled 24 news claims from PolitiFact.com\footnote{https://www.politifact.com/}. Thus we have the veracity label and fact-checked
evidence written by professional fact-checkers. We follow LIAR-PLUS \cite{alhindi2018your} to collect the evidence of each news claim. Each of the Participants viewed 8 news claims, half of the news claims are fake news, the other half are real news. The news claim were selected through a pilot study with 72 US annotators included to avoid extreme political leaning, familiarity and perceived accuracy. Half of the claims were meant to appeal to people who lean politically left, and the other half were designed for those who lean politically right.

Participants were randomly assigned to the control group, model-generated counterfactual explanation (CF-E), or warning tag (WT) group. 

\begin{enumerate}
    \item \textbf{Pre-test (Control Phase):} All participants read four fake news claims and four true news claims. Participants are asked to indicate their familiarity using a five-point scale: \textit{Have you ever seen or heard about this claim?} (1 = Definitely not, 5 = Definitely yes) and perceived accuracy using a seven-point scale: \textit{To the best of your knowledge, how accurate is the claim?} ($-3$ = Definitely not accurate , 3 = Definitely accurate). As Confirmation bias has been found to influence users beliefs in news claims\cite{ling2020confirmation, knobloch2020confirmation}, we follow previous study to collect the participants confirmation bias on each news claims\cite{moravec2020appealing} by asking the participants perceived importance using a seven-point scale: \textit{Do you find the issue described in the article important?} (1 = Not important at all, 7 = Extremely important). Confirmation bias was measured by multiplying the Perceived accuracy and importance together, creating a scale from $-21$ to 21.

    \item \textbf{Reading Environment (Intervention Phase):} The human subjects were assigned to three groups in this stage: the control group, the CF-E group, and the WT group. Participants in the
	 control group did not see any fake news intervention method in this module. The subjects read the same 8 news claims as in the pre-test in this module. Participants in the intervention groups saw the fake news debunking strategy along with the fake news claim. Figure~\ref{fig:interface} shows the interface of our intervention strategy with the claims.
  
    \item \textbf{Questionnaire:} We solicited participants' opinions on the fact-checked debunking strategy. We asked the participant to choose perceived fake news debunking strategy  using a five-point scale: \textit{In the previous module, do you see any fake news debunking strategy?}(1 = Definitely not, 5 = Definitely yes).
    Other multi-choice questions ask about the helpfulness, the overall experience of the survey. We administered the questionnaire in this stage to allow the
	 participants to rest after they saw the fake news debunking
	 strategy in the intervention module.
  
    \item \textbf{Post-test} Subjects saw the same news claims
	 from the pre-test module. We again enquired about the perceived accuracy of the news claims
	 to determine whether the fake news debunking strategy flip the participants' initial stance on each claim. Furthermore, we ask the reason of the perceived accuracy by a multi-choice question: \textit{Why do you choose the answer of the previous question?} (I choose this answer base on my previous knowledge, I choose this answer because I saw the tag/ explanation, I choose this answer because I searched online, others - text field).

   \newpage
    \item \textbf{Long-term test} Since 24 hour of has been used in cognitive psychology and psychology science literature to evaluate human long-term memory \cite{ rivera2022rate, frith2017randomized, chan2006retrieval, chan2010long, nairne1992loss}, we follow previous studies of 24 hour setting to examine the long-term effect of the fake news intervention methods. After a 24-hour wait, we invited the human subjects back to enquire about the perceived accuracy of the news claims, same with the post-test. This yielded an understanding of the long-term effectiveness of the fact-checked debunking strategy. 
    
\end{enumerate}

\subsection{Quality Control and Payment}

We use Prolific and calculate pay on a rate of $\$8$/ hour, which is above the federal minimum wage in the United States. The news articles used in our research were collected from PolitiFact.com, a website primarily featuring news from the United States. Therefore, we required our annotators to be located in the United States. This was done to ensure that the annotators had a cultural and contextual understanding of the news items, which is crucial for understanding the news we presented and the counterfactual explanations. For each of the question, we require a minimum reading and selection time of 5 seconds until the submission botton shows up. 
\subsection{Demographic of Participants}
\input{emnlp2023-latex/table/demographic}
\input{emnlp2023-latex/table/fake_claims}
